# Supplementary material for: Autonomous Maxwell's demon in a cavity QED system
Source: arXiv:2001.07445 source file (2020-07-03)
Supplement: Supplementary file 1 [file Supplementary.pdf]

# Supplementary information: Autonomous Maxwell's demon in a cavity QED system

Baldo-Luis Najera-Santos,[1] Patrice A. Camati,[2] Valentin Métillon,[1] Michel Brune,[1] Jean-Michel Raimond,[1] Alexia Auffèves,[2] and Igor Dotsenko[1]

[1]*Laboratoire Kastler Brossel, Collège de France, CNRS, ENS-Université PSL, Sorbonne Université, 11 place Marcelin Berthelot, F-75231 Paris, France*
[2]*Université Grenoble Alpes, CNRS, Grenoble INP, Institut Néel, 38000 Grenoble, France*
(Dated: June 26, 2020)

Section I presents the derivation of the entropy conservation in a qubit-demon-cavity system, given by Eq. (2) of the main paper. In Section II we describe the basic experimental protocol in terms of quantum logic circuit. In Sections III we give the definition of a cavity thermal field, explain its experimental preparation and control, and present the maximum-likelihood reconstruction of its photon-number distribution. Section IV presents a thermal state of a two-level atom and then show the measured populations of three atomic states, used for coding a qubit and a demon, depending on the initial state of the atom. Finally, in Section V we present a theoretical model describing our experimental protocol taking into account the main experimental imperfections, such as read-out efficiency, atomic relaxation, and detection errors.

## I. CONSERVATION OF ENTROPY

In order to obtain Eq. (2) of the main paper, we start from the following identity for the relative entropy (divergence):

$$\mathcal{D}\left(\hat{\rho}_{\mathsf{X}}||\hat{\mathcal{G}}_{\beta_{\mathsf{X}}}\right)=\beta_{\mathsf{X}}\left[\mathcal{U}\left(\hat{\rho}_{\mathsf{X}}\right)-\mathcal{F}^{\mathrm{eq}}_{\mathsf{X}}\right]-\mathcal{S}\left(\hat{\rho}_{\mathsf{X}}\right), \qquad (1)$$

where $\hat{\rho}_{\mathsf{X}}$ is an arbitrary state for the system, $\mathcal{U}_{\mathsf{X}}\equiv\mathcal{U}\left(\hat{\rho}_{\mathsf{X}}\right)=\mathrm{Tr}\left[\hat{H}_{\mathsf{X}}\hat{\rho}_{\mathsf{X}}\right]$ is the internal energy for some Hamiltonian $\hat{H}_{\mathsf{X}}$, $\hat{\mathcal{G}}_{\beta_{\mathsf{X}}}=e^{-\beta_{\mathsf{X}}\left(\hat{H}_{\mathsf{X}}-\mathcal{F}^{\mathrm{eq}}_{\mathsf{X}}\right)}$ is a Gibbs state, and $\mathcal{F}^{\mathrm{eq}}_{\mathsf{X}}=-\left(\beta_{\mathsf{X}}\right)^{-1}\ln\mathrm{Tr}\left[e^{-\beta_{\mathsf{X}}\hat{H}_{\mathsf{X}}}\right]$ is the equilibrium free energy. Applying this identity for two different times with the same reference Gibbs state ($\Delta\mathcal{F}^{\mathrm{eq}}_{\mathsf{X}}=0$) and taking their difference one obtains

$$\Delta\mathcal{S}_{\mathsf{X}}=\beta_{\mathsf{X}}\Delta\mathcal{U}_{\mathsf{X}}-\Delta\mathcal{D}_{\mathsf{X}}, \qquad (2)$$

after rearranging the terms. Considering the two instants of time to be before and after the feedback step and for the systems $\mathsf{X}\in\{\mathsf{Q},\mathsf{C}\}$, we substitute $\Delta\mathcal{S}_{\mathsf{X}}$ from Eq. (2) into $\Delta\mathcal{S}_{\mathsf{QC}}=\Delta\mathcal{S}_{\mathsf{Q}}+\Delta\mathcal{S}_{\mathsf{C}}-\Delta\mathcal{I}_{\mathsf{Q:C}}$, where $\mathcal{I}_{\mathsf{Q:C}}$ denotes the mutual information between two systems. After such a substitution and recognizing the following identity $\mathcal{D}\left(\hat{\rho}_{\mathsf{XY}}||\hat{\mathcal{G}}_{\beta_{\mathsf{X}}}\otimes\hat{\mathcal{G}}_{\beta_{\mathsf{Y}}}\right)=\mathcal{D}\left(\hat{\rho}_{\mathsf{X}}||\hat{\mathcal{G}}_{\beta_{\mathsf{X}}}\right)+\mathcal{D}\left(\hat{\rho}_{\mathsf{Y}}||\hat{\mathcal{G}}_{\beta_{\mathsf{Y}}}\right)+\mathcal{I}_{\mathsf{X:Y}}$ one finally arrives at

$$\Delta\mathcal{S}_{\mathsf{QC}}=\beta_{\mathsf{Q}}\Delta\mathcal{U}_{\mathsf{Q}}+\beta_{\mathsf{C}}\Delta\mathcal{U}_{\mathsf{C}}-\Delta\mathcal{D}_{\mathsf{QC}}. \qquad (3)$$

This is one way to write the entropy change of the thermodynamic system QC during the feedback step. The only assumption behind Eq. (3) was that there is no interaction Hamiltonian before and after the feedback step. This is naturally accomplished in our setup since the Rydberg atom passes through the cavity, hence effectively turning the interaction on, while inside the cavity, and then off, after leaving the cavity.

Now, we write the same entropy change in a different form, relating it to the demon D. This is easily achieved by rewriting the definition of mutual information $\mathcal{I}_{\mathsf{QC:D}}$ for the partition QC:D of our system, obtaining

$$\Delta\mathcal{S}_{\mathsf{QC}}=\Delta\mathcal{S}_{\mathsf{QDC}}-\Delta\mathcal{S}_{\mathsf{D}}+\Delta\mathcal{I}_{\mathsf{QC:D}}. \qquad (4)$$

Before we put these equations together, we state some properties of the feedback step of our protocol that can be checked to be true and that are necessary for the derivation:

(i) since there is no driving on any of the subsystems during the feedback step, the first law of thermodynamics allows us to identify $\Delta\mathcal{U}_{\mathsf{X}}=\mathcal{Q}_{\mathsf{X}}$ as the heat absorbed by the system X;

(ii) the total energy change is conserved (isolated unitary evolution), i.e., $\Delta\mathcal{U}_{\mathsf{QDC}}=\Delta\mathcal{U}_{\mathsf{Q}}+\Delta\mathcal{U}_{\mathsf{D}}+\Delta\mathcal{U}_{\mathsf{C}}=0$;

(iii) the total entropy is conserved (unitary process), i.e., $\Delta\mathcal{S}_{\mathsf{QDC}}=0$;

(iv) the reduced demon state $\hat{\rho}_{\mathsf{D}}$ does not change during the feedback step and hence its energy and entropy are conserved, i.e., $\Delta\mathcal{U}_{\mathsf{D}}=0$ and $\Delta\mathcal{S}_{\mathsf{D}}=0$;

(v) initial state of the qubit and the cavity before the feedback step are the Gibbs state, hence $\Delta\mathcal{D}_{\mathsf{QC}}=\mathcal{D}_{\mathsf{QC}}$, i.e., the change is given by the final divergence only.

Property (iv) is true because the demon state after the read-out step is diagonal in the computational basis which is also the basis for the controlled unitary in Fig. S1. From properties (i) and (iv) one can see that no energy is transferred to the demon. Together with (ii) it results in $\mathcal{Q}_{\mathsf{C}}=-\mathcal{Q}_{\mathsf{Q}}$, meaning that the heat absorbed

by the qubit is the same as the heat given off by the cavity and vice versa. With properties (i), (ii), (iv), and (v), Eq. (3) becomes

$$\Delta\mathcal{S}_{\mathsf{QC}} = \delta\beta\mathcal{Q}_{\mathsf{C}} - \mathcal{D}_{\mathsf{QC}}, \tag{5}$$

where $\delta\beta = \beta_{\mathsf{C}} - \beta_{\mathsf{Q}}$. With properties (iii) and (iv), Eq. (4) becomes

$$\Delta\mathcal{S}_{\mathsf{QC}} = \Delta\mathcal{I}_{\mathsf{QC:D}}. \tag{6}$$

Together, Eqs. (5) and (6) give Eq. (2) of the main paper.

## II. LOGICAL STATES AND EFFECTIVE QUANTUM CIRCUIT

In order to independently describe the qubit and demon states, we map the three atomic levels $\{|e\rangle, |g\rangle, |f\rangle\}$ into a subspace of a two-qubit Hilbert space of Q and D as

$$\begin{aligned} |e\rangle &= |1_{\mathsf{Q}}\rangle \otimes |0_{\mathsf{D}}\rangle, \\ |g\rangle &= |0_{\mathsf{Q}}\rangle \otimes |0_{\mathsf{D}}\rangle, \\ |f\rangle &= |0_{\mathsf{Q}}\rangle \otimes |1_{\mathsf{D}}\rangle. \end{aligned} \tag{7}$$

We refer to this "logical basis" as qubit-demon, or QD basis for short. Since the density operator describing the initial state of the atom is $\hat{\rho}_{\mathcal{A}}^{(0)} = |g\rangle\langle g|$, the initial QD state is $\hat{\rho}_{\mathsf{QD}}^{(0)} = |0_{\mathsf{Q}}0_{\mathsf{D}}\rangle\langle 0_{\mathsf{Q}}0_{\mathsf{D}}|$.

Figure S1 shows an effective quantum circuit describing the autonomous operation of our Maxwell's demon. Initial states of C and Q are thermal, while the demon D is initially in its ground state. The read-out process is realized by a controlled-NOT gate between Q and D. The feedback is modelled by a controlled unitary operation $\hat{\mathcal{U}}_{\text{fb}}$ between C and Q conditioned on D. Note that both controlled gates are conditioned on a control qubit in $|0\rangle$ state. In Section V we describe in detail each element of this circuit.

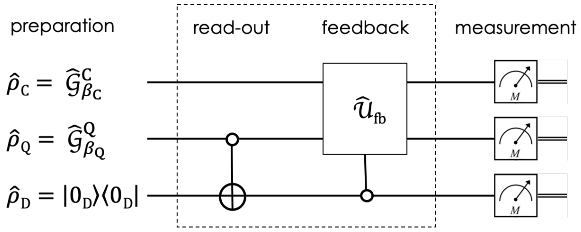


FIG. S1. Effective quantum circuit describing the autonomous Maxwell's demon operation. The operations in a dashed box are unitary. The final measurement is used to reconstruct the system's state and then to compute all thermodynamic quantities.

Note also that all states in the current work have no coherences and are thus diagonal in energy basis. However, for the sake of generality, we continue to use density matrices ($\hat{\rho}$) instead of state populations ($\rho_{ii}$) when describing state evolutions and calculating entropic quantities. Finally, the fourth state of the QD system, $|1_{\mathsf{Q}}\rangle \otimes |1_{\mathsf{D}}\rangle$, is never populated and, thus, do not need to be coded onto the atom. Since both physical and logical states of this mapping are orthogonal in their respective Hilbert spaces, these two sets are isomorphic and therefore their mapping is bijective with no loss of information or change in entropy.

## III. CAVITY THERMAL FIELD

### Definition

The concept of temperature in quantum thermodynamics is very similar to its counterpart in statistical physics. According to Boltzmann, the probability of finding the system, that is in thermal equilibrium at temperature $T$, in level $|m\rangle$ decreases exponentially with the level energy $E_m$:

$$P(m) = \mathcal{Z}^{-1} \exp\left(-\frac{E_m}{k_{\text{B}}T}\right), \tag{8}$$

where the normalization parameter $\mathcal{Z}$ is the partition function defined as

$$\mathcal{Z} = \sum_{m=0}^{\infty} \exp\left(-\frac{E_m}{k_{\text{B}}T}\right). \tag{9}$$

In the following, we use an inverse temperature defined as $\beta = (k_{\text{B}}T)^{-1}$.

For a cavity C at temperature $\beta_{\mathsf{C}}$ and with resonant frequency $\omega_{\mathsf{C}}/2\pi = 51$ GHz, we get a thermal photon-number distribution

$$P^{\mathsf{C}}_{\beta_{\mathsf{C}}}(n) = (1 - e^{-\hbar\omega_{\mathsf{C}}\beta_{\mathsf{C}}})\, e^{-n\hbar\omega_{\mathsf{C}}\beta_{\mathsf{C}}} = \frac{{n_{\text{th}}}^n}{(1+n_{\text{th}})^{n+1}}, \tag{10}$$

with the thermal (mean) photon number

$$n_{\text{th}} = \frac{1}{e^{\hbar\omega_{\mathsf{C}}\beta_{\mathsf{C}}} - 1}. \tag{11}$$

The cavity thermal field and the corresponding inverse temperature, respectively, read

$$\hat{\mathcal{G}}^{\mathsf{C}}_{\beta_{\mathsf{C}}} = \sum_{n=0}^{\infty} P^{\mathsf{C}}_{\beta_{\mathsf{C}}}(n)\, |n\rangle\langle n|, \tag{12}$$

$$\beta_{\mathsf{C}} = (\hbar\omega_{\mathsf{C}})^{-1} \ln\left(\frac{1+n_{\text{th}}}{n_{\text{th}}}\right). \tag{13}$$

### Preparation

Each experimental sequence starts by erasing the residual microwave field in the cavity C with a sequence of

several tens of atoms prepared in the ground state $|g\rangle$ and resonantly absorbing all photons from C. To prepare a thermal field, we inject into the empty C a series of coherent microwave pulses generated by the microwave source $\mathsf{C_C}$. All injections have equal absolute amplitude $\alpha$ and duration $\tau$, but have different and random phases. During these injections the cavity field undergoes a random walk in phase space, starting from the space origin. The average field amplitude after $N_{\rm inj}$ injections, i.e., after a total injection time $t_{\rm inj} = N_{\rm inj}\tau$, is given by

$$\alpha_{\rm inj} = \alpha\sqrt{N_{\rm inj}} = \alpha\sqrt{\frac{t_{\rm inj}}{\tau}}. \tag{14}$$

Consequently, the mean photon number $\langle n\rangle = \alpha_{\rm inj}^2$ is not expected to grow quadratically with time, as it does for the coherent pumping, but rather linearly. After a large number of injections, the photon-number distribution $P(n)$ converges to the Boltzmann distribution with a thermal photon number $n_{\rm th}$ equal to the mean photon number: $n_{\rm th} \approx \langle n\rangle$. We have checked numerically, that after only $N_{\rm inj} = 10$ injections with an amplitude $\alpha < 0.1$ photons, the built-up distribution is close to the Boltzmann one. A more reliable verification of the successful thermal field preparation is done experimentally, see below.

### Calibration

The thermal field injection is experimentally precalibrated using the Ramsey interferometer $\mathsf{R_1}$-$\mathsf{R_2}$ [1]. The method is similar to the one presented in Ref. [2, Appendix A.3]. Each photon number state in the cavity shifts the Ramsey fringe in a well-defined way depending on the interferometer settings (i.e., dephasing per photon). The Ramsey signal, i.e., the population transfer of the QND atoms from their initial state $|g\rangle$ to $|e\rangle$, depends on the photon number $n$ as

$$p_e(n,\phi_r) = y_0 + \frac{c}{2}\cos\left(n\phi_0 + \phi_r\right). \tag{15}$$

The offset $y_0$ and the contrast $c$ of the Ramsey fringes can be calibrated independently on the vacuum field. For the cavity field with a photon-number distribution $P(n)$ the Ramsey signal is a sum of individual photon number contributions:

$$p_e(\phi_r) = \sum_{n=0}^{\infty} p_e(n,\phi_r)P(n). \tag{16}$$

In the case of a coherent field of amplitude $\beta$ (i.e., constant phase injections), $P(n)$ reads

$$P(n) = e^{-\langle n\rangle}\frac{\langle n\rangle^n}{n!} \tag{17}$$

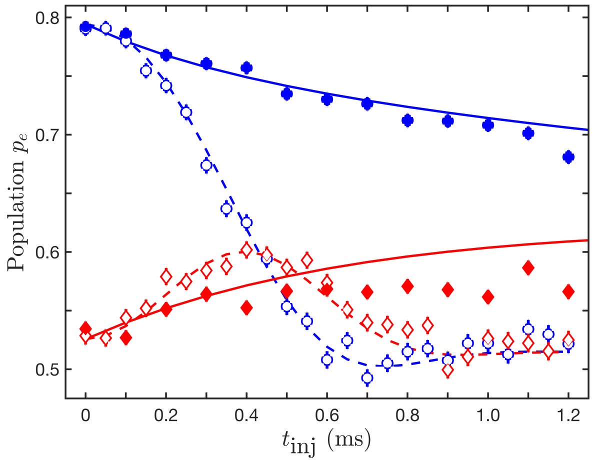

FIG. S2. Calibration of the injection amplitude with Ramsey fringes. Points are experimental, lines are fits. Blue (red) is for the Ramsey phase $\phi_{r1} = 0$ ($\phi_{r2} = \pi/2$). Full points and solid lines are for the thermal field. Open points and dashed lines are for the coherent field. The fitted parameters are $\gamma_{\rm coh} = 2.1\,{\rm ms}^{-1}$ and $\gamma_{\rm th} = 0.39\,{\rm ms}^{-1}$.

with $\langle n\rangle = |\beta|^2$. The total Ramsey signal is then

$$p_e^{\rm coh} = y_0 + \frac{c}{2}\,e^{(\cos\phi_0 - 1)\langle n\rangle}\cos\left(\phi_r + \langle n\rangle\sin\phi_0\right). \tag{18}$$

Assuming that $\langle n\rangle = \gamma_{\rm coh}\,t_{\rm inj}^2$, we get the theoretical dependence of $p_e^{\rm coh}$ on $t_{\rm inj}$.

For the thermal field, $P(n)$ is given by (10) and the Ramsey signal is

$$p_e^{\rm th} = y_0 + \frac{c}{2}\frac{(1+n_{\rm th})\cos\phi_r - n_{\rm th}\cos(\phi_r - \phi_0)}{(1+n_{\rm th}(1-\cos\phi_0))^2 + (n_{\rm th}\sin\phi_0)^2}. \tag{19}$$

If we assume that $n_{\rm th} = \gamma_{\rm th}\,t_{\rm inj}$, we obtain the dependence of $p_e^{\rm th}$ on $t_{\rm inj}$.

We use here the same interferometer settings as those used for the cavity state reconstruction in the main paper. Namely, the dephasing per photon is $\phi_0 = \pi/2$ and we use two interleaved ensembles of QND atoms with Ramsey phases $\phi_{r1} = 0$ and $\phi_{r2} = \pi/2$ aligned to maximize the atom population $p_e$ in state $|e\rangle$ for the vacuum state and for the one-photon state, respectively. We record the dependence of the Ramsey signal (i.e., atomic population) on the injection duration. By comparing it to the theoretical variation for the Poisson (i.e., for a coherent field) and Boltzmann (i.e., for a thermal field) photon-number distribution, we obtain the calibrated mean photon numbers.

Figure S2 shows $p_e^{\rm th}(t_{\rm inj})$ and $p_e^{\rm coh}(t_{\rm inj})$, measured and fitted, for two Ramsey phases (blue and red for $\phi_{r1}$ and $\phi_{r2}$, respectively). Open points and dashed lines are for the coherent field, while full points and solid lines are for the thermal field. The points are the measured population transfer and the lines are the corresponding fits

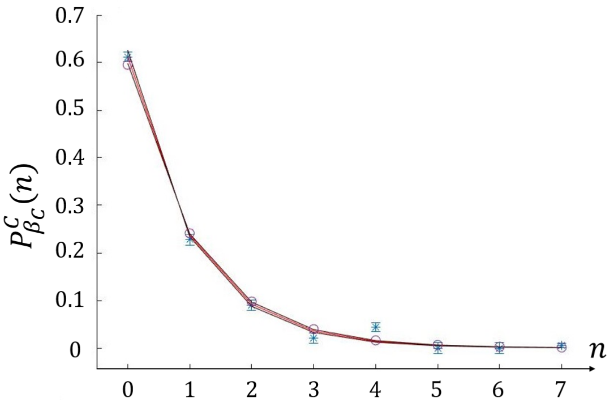


FIG. S3. Reconstructed cavity thermal state $P^{\mathsf{C}}_{\beta_{\mathsf{C}}}(n)$. Blue points are reconstructed populations. Solid line with open circles is a fit with a Boltzmann distribution (10), given $n_{\rm th} = 0.63 \pm 0.04$ photons.

with (18) and (19). For the thermal field, the injection phase is randomly changed every 0.1 ms. From this quick measurement, which requires no sophisticated state reconstruction, we get a value of $\gamma_{\rm th} = 0.39\,{\rm ms}^{-1}$ and thus $n_{\rm th} = 0.39$ photons after 1 ms injection with the microwave source power used in Fig. S2.

### Reconstruction

We reconstruct the photon-number distribution of the thermal field with our quantum state tomography method [3]. Figure S3 shows the reconstructed $P(n)$ after the incoherent pumping (i.e., with random phases) of $\mathsf{C}$ with 10 weak injections. The data fit to the thermal field distribution results in $n_{\rm th} = 0.63 \pm 0.04$ photons and, according to (13), in $\beta_{\mathsf{C}} = (0.95 \pm 0.04)(\hbar\omega_{\mathsf{C}})^{-1}$ and $T_{\mathsf{C}} = 2.6 \pm 0.1$ K. This value is used in all experimental sequences presented in the paper. The residual noise on $P(n)$ for higher photon numbers ($n \geq 4$) results in the mean photon number $\langle n \rangle = 0.68$ slightly higher than the fitted $n_{\rm th}$.

We repeat the same analysis for different injection times $t_{\rm inj}$, i.e., after different number of injections $N_{\rm inj}$ of 0.1 ms duration. Figure S4 presents the dependence of the reconstructed $n_{\rm th}$ on $t_{\rm inj}$. Note that the power of the microwave source $\mathsf{S}_{\mathsf{C}}$ in this test is set higher than that used in the main experiment. Starting from about 4 injections, $n_{\rm th}$ grows linearly, as expected from the random walk in the phase space.

For the experiments presented in the paper, we apply $N_{\rm inj} = 10$ weak injections of $\tau = 0.1$ ms duration, resulting in $t_{\rm inj} = 1$ ms. The power of the microwave source $\mathsf{S}_{\mathsf{C}}$ is set to have $n_{\rm th} = 0.63$ photons.

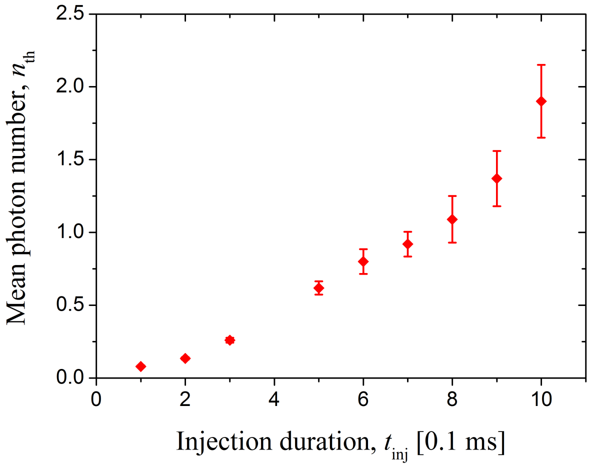


FIG. S4. Mean photon number versus injection duration. The injection phase is randomly changed every 0.1 ms. Starting from $N_{\rm inj} \leq 3$ injections, the growth of $\langle n \rangle$ is close to linear. In the experiment, we use $N_{\rm inj} = 10$ injections to prepare a thermal field. For thermal fields with $\langle n \rangle > 1.5$ the current reconstruction with the Hilbert space dimension of 7 photons starts to produce inaccurate state estimation.

## IV. ATOMIC STATE MANIPULATIONS

### Thermal state

We consider a qubit with states $|0\rangle$ and $|1\rangle$. The population of its excited state $|1\rangle$ at temperature $\beta_{\mathsf{Q}}$ reads

$$n_{\mathsf{Q}} \equiv P^{\mathsf{Q}}_{\beta_{\mathsf{Q}}}(1) = \frac{1}{\exp(\hbar\omega_{\mathsf{Q}}\beta_{\mathsf{Q}}) + 1}, \tag{20}$$

where $n_{\mathsf{Q}}$ is the qubit occupancy. The qubit thermal state is then a statistical mixture of two pure states with the corresponding probabilities:

$$\hat{\mathcal{G}}^{\mathsf{Q}}_{\beta_{\mathsf{Q}}} = P^{\mathsf{Q}}_{\beta_{\mathsf{Q}}}(0)\,|0\rangle\langle 0| + P^{\mathsf{Q}}_{\beta_{\mathsf{Q}}}(1)\,|1\rangle\langle 1|, \tag{21}$$

where the ground state population is $P^{\mathsf{Q}}_{\beta_{\mathsf{Q}}}(0) = 1 - P^{\mathsf{Q}}_{\beta_{\mathsf{Q}}}(1)$. Using (20), we get for the inverse temperature

$$\beta_{\mathsf{Q}} = (\hbar\omega_{\mathsf{Q}})^{-1} \ln\left(\frac{1 - n_{\mathsf{Q}}}{n_{\mathsf{Q}}}\right). \tag{22}$$

### Initial state

We set the initial inverse temperature $\beta_{\mathsf{Q}}$ of our atomic qubit $\mathsf{Q}$ (states $|g\rangle$ and $|e\rangle$) with a resonant microwave pulse applied to $\mathsf{Q}$ in state $|g\rangle$ by microwave source $\mathsf{S}_{eg}$. The excited state population oscillates with the pulse duration $t_{\mathsf{Q}}$ as

$$n_{\mathsf{Q}} \equiv P(e) = \pi_0 - \frac{c_{\mathsf{Q}}}{2}\cos\left(\Omega t_{\mathsf{Q}}\right). \tag{23}$$

We omit in the following the subscripts and superscripts $\beta_{\mathsf{Q}}$ and $\mathsf{Q}$ for the atomic populations where obvious. The offset $\pi_0$ and the contrast $c_{\mathsf{Q}}$ account for the imperfection of these Rabi oscillations (spacial dispersion of atoms in an atomic sample, microwave field inhomogeneity, detection errors, etc). The Rabi frequency $\Omega$ depends on the microwave power. Each $P(e)$ corresponds to a unique qubit temperature $\beta_{\mathsf{Q}}$ given by (22). Thus, we control $\beta_{\mathsf{Q}}$ by choosing the pulse duration $t_{\mathsf{Q}}$.

Figure S5(a) presents the probability $P(a)$ to detect the atom in one of its three states ($a \in \{f, g, e\}$) depending on the pulse duration $t_{\mathsf{Q}}$. The observed Rabi frequency is $\Omega/2\pi = 77$ kHz. For $t_{\mathsf{Q}} = 0$ some atoms are detected in $|e\rangle$, because of the state discrimination error $\eta$ of our nonideal detector. We also observe some atoms in $|f\rangle$, because of the combination of $\eta$ and the atomic spontaneous relaxation from $|g\rangle$ to $|f\rangle$ between the state preparation and detection. As expected, $P(f)$ decreases together with $P(g)$.

### Qubit-cavity energy exchange

Figure S5(b) shows the atomic populations $P(a)$ after the adiabatic passage transfer between $\mathsf{Q}$ and $\mathsf{C}$. At a half Rabi period ($t_{\mathsf{Q}} \approx 6.5\,\mu$s), $P(g)$ and $P(e)$ are opposite to those in Fig. S5(a), since $\mathsf{Q}$ has emitted a photon into $\mathsf{C}$, passing from $|e\rangle$ to $|g\rangle$. The probability for $\mathsf{Q}$ in $|g\rangle$ to absorb a photon equals the probability to have at least 1 photon in $\mathsf{C}$. Therefore, for $t_{\mathsf{Q}} = 0$ and $\mathsf{Q}$ prepared mainly in $|g\rangle$, $P^{\mathsf{Q}}(e|t_{\mathsf{Q}} = 0) = 1 - P^{\mathsf{C}}(0)$ and $P^{\mathsf{Q}}(g|t_{\mathsf{Q}} = 0) = P^{\mathsf{C}}(0)$, where $P^{\mathsf{C}}(0)$ is the probability of the vacuum field in $\mathsf{C}$. Here, $\beta_{\mathsf{C}} = 0.90(\hbar\omega_{\mathsf{C}})^{-1}$, resulting in $P^{\mathsf{C}}(0) = 0.59$, which is close to the observed value of $P^{\mathsf{Q}}(e|t_{\mathsf{Q}} = 0) = 0.52 \pm 0.04$ if considering the reduced contrast $c$ of the Rabi oscillations.

### Demon read-out

Now, we consider the effect of the demon read-out onto the energy exchange between $\mathsf{Q}$ and $\mathsf{C}$, at temperatures $\beta_{\mathsf{Q}}(t_{\mathsf{Q}})$ and $\beta_{\mathsf{C}}(t_{\mathrm{inj}})$. Unlike the previous case, the atom is transferred from $|g\rangle$ to $|f\rangle$ with a demon read-out pulse, before the $\mathsf{Q}$-$\mathsf{C}$ energy exchange. Figure S5(c) shows the state of the atom, after read-out and before the interaction. As expected, the levels $|g\rangle$ and $|f\rangle$ have exchanged their populations, compared to Fig. S5(a). The remaining population $P(g)$ for $t_{\mathrm{inj}} = 0$ reveals the limited demon pulse efficiency, $\eta_{\mathsf{D}} \approx 0.95$, due to the inhomogeneity of the radiating microwave field.

Figure S5(d) displays the final state of the atoms after the feedback (i.e., adiabatic passage between $\mathsf{Q}$ and $\mathsf{C}$). The population $P(f)$ remains the same as in Fig. S5(c), since the $|g\rangle \to |f\rangle$ transition is far detuned from the cavity frequency. Moreover, we observe an almost perfect transfer from $|e\rangle$ to $|g\rangle$, showing the high efficiency of the adiabatic passage.

The current readout process is implemented by transferring the atomic population between two non-degenerate levels. However, since this transfer is induced by a strong classical coherent field, the atom (and, thus, the system in total) does not get entangled with the external field. Consequently, there is no information (entropy) flow outside of the system and all entropy analysis is valid. On the other hand, the energy of the field mode does increase on average. In principle, it could be used at the very end of our protocol to reset the demon $\mathsf{D}$ back to its initial state.

## V. THEORETICAL MODEL

In this chapter we present a theoretical model describing the evolution of our QDC system during the experimental sequence and taking into account the main experimental imperfections which affect the measurement results. This model is used for all theoretical curves in the main paper. Note that for the bijective state mapping between physical and logical states implemented here, all QDC operators are defined in a unique way.

### Thermal state preparation

We model the qubit preparation in the thermal state using the following unitary transformation $\hat{\mathcal{U}}_{\mathrm{th}}$:

$$\hat{\mathcal{U}}_{\mathrm{th}}(\theta) = \sqrt{1 - n_{\mathsf{Q}}}\,\hat{I}_{\mathsf{Q}} - i\,\sqrt{n_{\mathsf{Q}}}\,\hat{\sigma}_Y = \begin{pmatrix} \sqrt{1-n_{\mathsf{Q}}} & -\sqrt{n_{\mathsf{Q}}} \\ \sqrt{n_{\mathsf{Q}}} & \sqrt{1-n_{\mathsf{Q}}} \end{pmatrix}, \tag{24}$$

where $n_{\mathsf{Q}}$ is given by (23) and $\hat{I}_{\mathsf{Q}} = \hat{I}_{\mathsf{D}} = \hat{I}_2$ is the identity operator in a two-dimensional Hilbert space. The QD density matrix transforms according to

$$\begin{aligned}\hat{\rho}^{\mathrm{th}}_{\mathsf{QD}} &= \left(\hat{\mathcal{U}}_{\mathrm{th}} \otimes \hat{I}_{\mathsf{D}}\right) \hat{\rho}^{(0)}_{\mathsf{QD}} \left(\hat{\mathcal{U}}^{\dagger}_{\mathrm{th}} \otimes \hat{I}_{\mathsf{D}}\right) \\ &= n_{\mathsf{Q}} |1_{\mathsf{Q}}0_{\mathsf{D}}\rangle\langle 1_{\mathsf{Q}}0_{\mathsf{D}}| + (1 - n_{\mathsf{Q}})\,|0_{\mathsf{Q}}0_{\mathsf{D}}\rangle\langle 0_{\mathsf{Q}}0_{\mathsf{D}}| \\ &\quad - \sqrt{n_{\mathsf{Q}}(1-n_{\mathsf{Q}})}\big\{|1_{\mathsf{Q}}0_{\mathsf{D}}\rangle\langle 0_{\mathsf{Q}}0_{\mathsf{D}}| + |0_{\mathsf{Q}}0_{\mathsf{D}}\rangle\langle 1_{\mathsf{Q}}0_{\mathsf{D}}|\big\}.\end{aligned} \tag{25}$$

Although the qubit has non-vanishing coherences, we are not able to track them all along the experiment, and they are averaged out over several protocol repetitions. Neglecting the coherence, expression (25) simplifies to

$$\hat{\rho}^{\mathrm{th}}_{\mathsf{QD}} = n_{\mathsf{Q}}\,|1_{\mathsf{Q}}0_{\mathsf{D}}\rangle\langle 1_{\mathsf{Q}}0_{\mathsf{D}}| + (1 - n_{\mathsf{Q}})\,|0_{\mathsf{Q}}0_{\mathsf{D}}\rangle\langle 0_{\mathsf{Q}}0_{\mathsf{D}}|. \tag{26}$$

The initial state of the cavity $\mathsf{C}$ is a thermal state $\hat{\mathcal{G}}^{\mathsf{C}}_{\beta_{\mathsf{C}}}$ with temperature $\beta_{\mathsf{C}}$ given by (12). Thus, the initial joint QDC density matrix reads

$$\hat{\rho}^{\mathrm{th}}_{\mathsf{QDC}} = \hat{\rho}^{\mathrm{th}}_{\mathsf{QD}} \otimes \hat{\mathcal{G}}^{\mathsf{C}}_{\beta_{\mathsf{C}}}. \tag{27}$$

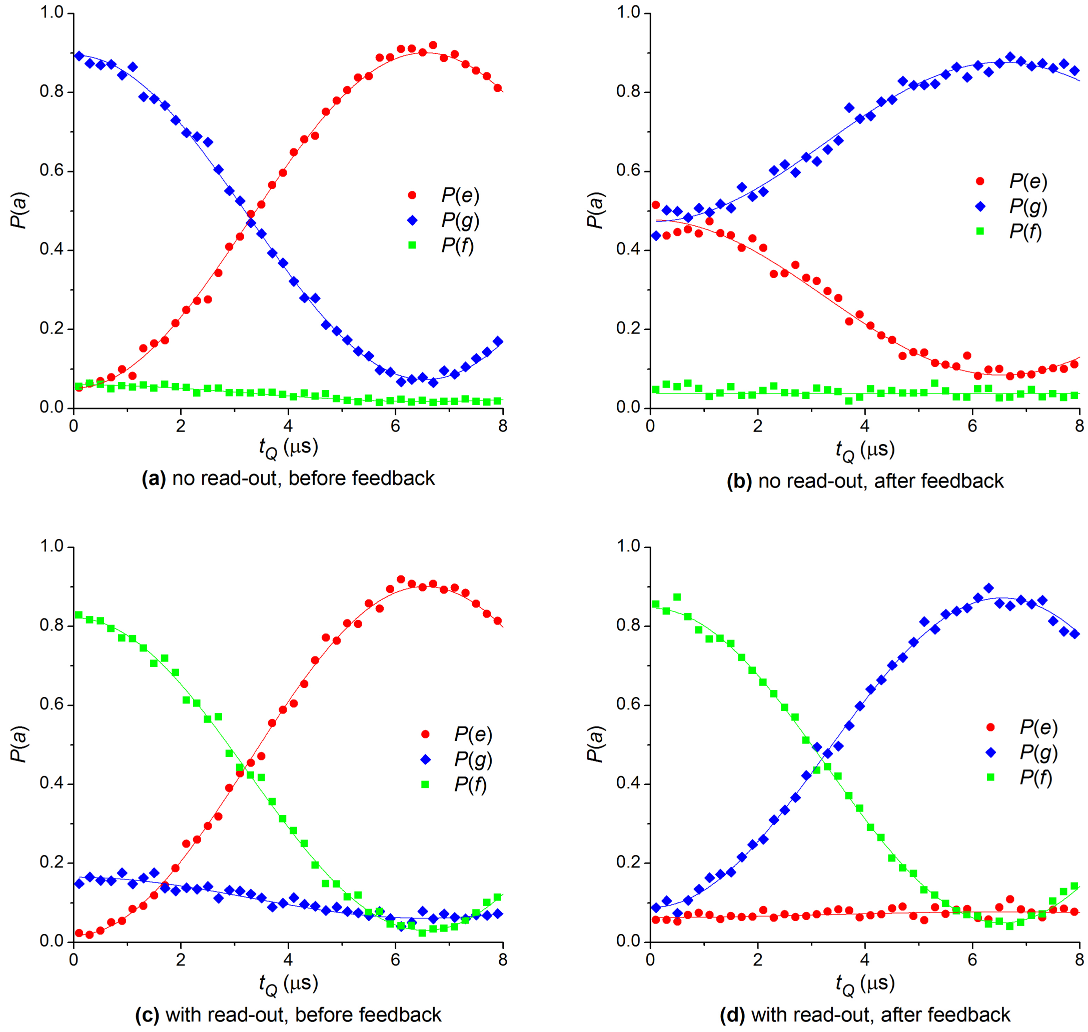


FIG. S5. Population of the atomic states, with and without demon read-out, versus the duration of the $|g\rangle \to |e\rangle$ microwave pulse before and after feedback (energy exchange). The atom is initially in state $|g\rangle$. The points represent experimental probabilities of atomic detection in $|e\rangle$ (red), $|g\rangle$ (blue), and $|f\rangle$ (green). The lines are sine fits.

### Demon read-out

The *read-out* step is implemented by a unitary transformation $\hat{\mathcal{U}}_{\rm rd}$:

$$\hat{\mathcal{U}}_{\rm rd} = |1_{\sf Q}\rangle\langle 1_{\sf Q}| \otimes \hat{I}_{\sf D} - i\,|0_{\sf Q}\rangle\langle 0_{\sf Q}| \otimes \hat{\sigma}_{\sf Y} \tag{28}$$

The limited efficiency $\eta_{\sf D}$ of our imperfect read-out is taken into account by mixing two possible evolutions: successful $\hat{\mathcal{U}}_{\rm rd}$ with probability $\eta_{\sf D}$ and unsuccessful $\hat{I}_{\sf Q} \otimes \hat{I}_{\sf D}$ with probability $(1-\eta_{\sf D})$. The QD density matrix is then transformed according to

$$\begin{aligned}\hat{\rho}^{\rm rd}_{\sf QD} &= \eta_{\sf D}\,(\hat{\mathcal{U}}_{\rm rd}\,\hat{\rho}^{\rm th}_{\sf QD}\,\hat{\mathcal{U}}^{\dagger}_{\rm rd}) + (1-\eta_{\sf D})\hat{\rho}^{\rm th}_{\sf QD} \\ &= n_{\sf Q}\,|1_{\sf Q}0_{\sf D}\rangle\langle 1_{\sf Q}0_{\sf D}| \\ &\quad +(1-\eta_{\sf D})(1-n_{\sf Q})\,|0_{\sf Q}0_{\sf D}\rangle\langle 0_{\sf Q}0_{\sf D}| \\ &\quad +\eta_{\sf D}(1-n_{\sf Q})\,|0_{\sf Q}1_{\sf D}\rangle\langle 0_{\sf Q}1_{\sf D}| \end{aligned}\tag{29}$$

and the QDC density matrix is

$$\hat{\rho}^{\rm rd}_{\sf QDC} = \hat{\rho}^{\rm rd}_{\sf QD} \otimes \hat{\mathcal{G}}^{\sf C}_{\beta_{\sf C}}. \tag{30}$$

### Feedback operation

The feedback operation controlling the heat exchange is realized with the adiabatic population transfer between Q and C. The calibrated efficiency is closed to unity. This operation transforms the QDC joint state as

$$\hat{\rho}^{\rm fb}_{\sf QDC} = \hat{\mathcal{U}}_{\rm fb}\,\hat{\rho}^{\rm rd}_{\sf QDC}\,\hat{\mathcal{U}}^{\dagger}_{\rm fb}. \tag{31}$$

where the unitary transformation $\hat{\mathcal{U}}_{\rm fb}$ is modelled by

$$\begin{aligned}\hat{\mathcal{U}}_{\rm fb} = \hat{\sigma}_{-} &\otimes |0_{\sf D}\rangle\langle 0_{\sf D}| \otimes \hat{b}_{+} + \hat{\sigma}_{+} \otimes |0_{\sf D}\rangle\langle 0_{\sf D}| \otimes \hat{b}_{-} \\ &+|0_{\sf Q}\rangle\langle 0_{\sf Q}| \otimes |0_{\sf D}\rangle\langle 0_{\sf D}| \otimes |0_{\sf C}\rangle\langle 0_{\sf C}| \\ &+\hat{I}_{\sf Q} \otimes |1_{\sf D}\rangle\langle 1_{\sf D}| \otimes \hat{I}_{\sf C}. \end{aligned}\tag{32}$$

Here, we have defined a set of cavity and qubit operators:

$$\hat{b}_+|n\rangle = |n+1\rangle,\;\; \hat{b}_-\,|n\rangle = |n-1\rangle,\;\; \hat{b}_+ = \hat{b}_-^\dagger;$$
$$\hat{\sigma}_+|0\rangle = |1\rangle,\;\; \hat{\sigma}_-\,|1\rangle = |0\rangle,\;\; \hat{\sigma}_+ = \hat{\sigma}_-^\dagger. \qquad (33)$$

The first and second terms in (32) describe the energy transfer from $\mathsf{Q}$ to $\mathsf{C}$ and from $\mathsf{C}$ to $\mathsf{Q}$, respectively. The third term accounts for the case when both $\mathsf{Q}$ and $\mathsf{C}$ are in their ground states and no heat exchange is thus possible. Finally, the fourth term corresponds to the situation when $\mathsf{D}$ actively prevents the heat exchange.

The joint $\mathsf{QC}$ population probabilities (i.e., the diagonal elements of the joint $\mathsf{QC}$ density matrix) after the feedback are given by

$$\begin{aligned}
P^{\varnothing}(n,1_\mathsf{Q}) &= (1-n_\mathsf{Q})P^\mathsf{C}(n+1) \qquad (34)\\
P^{\varnothing}(n,0_\mathsf{Q}) &= n_\mathsf{Q}P^\mathsf{C}(n-1)\\
P^{\varnothing}(0,0_\mathsf{Q}) &= (1-n_\mathsf{Q})P^\mathsf{C}(0)\\
P^{\mathrm{d}}(n,1_\mathsf{Q}) &= (1-\eta_\mathsf{D})\,(1-n_\mathsf{Q}\,)\,P^\mathsf{C}(n+1)\\
P^{\mathrm{d}}(n,0_\mathsf{Q}) &= n_\mathsf{Q}P^\mathsf{C}(n-1) + \eta_\mathsf{D}\,(1-n_\mathsf{Q})P^\mathsf{C}(n)\\
P^{\mathrm{d}}(0,0_\mathsf{Q}) &= (1-n_\mathsf{Q})P^\mathsf{C}(0)
\end{aligned}$$

where superscripts $\varnothing$ and d indicate the absence or presence of the demon read-out, respectively. The effect of $\mathsf{D}$ is essentially decreasing the heat loss of $\mathsf{C}$ by a factor of $(1-\eta_\mathsf{D})$, that is the probability for $\mathsf{D}$ to ignore $\mathsf{Q}$ in state $|0_\mathsf{Q}\rangle$.

### Atomic relaxation

The atomic levels are subjected to spontaneous relaxation to lower lying states. This relaxation is efficiently described by the set of rate equations:

$$\begin{aligned}
d\rho_{ee}/dt &= -\Gamma\rho_{ee},\\
d\rho_{gg}/dt &= -\Gamma\rho_{gg} + \Gamma\rho_{ee}, \qquad (35)\\
d\rho_{ff}/dt &= -\Gamma\rho_{ff} + \Gamma\rho_{gg}.
\end{aligned}$$

The relaxation times for the atomic levels $e$, $g$ and $f$ are about 33 ms, 30 ms and 27 ms, respectively. For the sake of simplicity, we consider the relaxation rate $\Gamma \approx (30\,\mathrm{ms})^{-1}$ to be the same for these levels and we neglect the possible thermal excitation of atoms due to thermal background radiation in our experiment. The solution to (35) is

$$\begin{aligned}
\rho_{ee} &= \rho_{ee,0}\,e^{-\Gamma t},\\
\rho_{gg} &= (\rho_{ee,0}\Gamma t + \rho_{gg,0})\,e^{-\Gamma t}, \qquad (36)\\
\rho_{ff} &= \left(\frac{1}{2}\rho_{ee,0}(\Gamma t)^2 + \rho_{gg,0}\Gamma t + \rho_{ff,0}\right)e^{-\Gamma t},
\end{aligned}$$

where subscript 0 refers to the initial atomic populations. The normalization condition $(\rho_{ee}+\rho_{gg}+\rho_{ff}=1)$ has to be taken into account by dividing (36) by the sum of its right-hand side terms.

The relaxation process occurs during all experimental sequence. The atomic velocity (250 m/s) and the fixed geometry of the experimental components (Ramsey zones, cavities, detector, etc) define the time intervals between the thermal state preparation, read-out, feedback and detection. We apply the atomic state transformation (36) to each of these intervals.

### Imperfect state detection

The imperfect state resolution of our detector leads to the effective mixing of the detected atomic states. We model it with the following Kraus map:

$$\hat{\rho} \to \sum_{a,b\in\{e,g,f\}} \hat{\mathcal{M}}_{a\to b}\,\hat{\rho}\,\hat{\mathcal{M}}^\dagger_{a\to b}, \qquad (37)$$

where the erroneous detection of an atomic state $|a\rangle$ as state $|b\rangle$ with probability $\epsilon_{a\to b}$ is described by

$$\hat{\mathcal{M}}_{a\to b} = \sqrt{\epsilon_{a\to b}}\;|b\rangle\langle a|. \qquad (38)$$

The closure relation implies that

$$\epsilon_{a\to a} = 1 - \sum_{b\neq a}\epsilon_{a\to b}. \qquad (39)$$

We have independently calibrated the detection errors and obtained the following values for $\epsilon_{a\to b}$:

$$\begin{aligned}
\epsilon_{e\to b} &= 0.02\,\delta_{b,g} + 0.98\,\delta_{b,e},\\
\epsilon_{g\to b} &= 0.07\,\delta_{b,e} + 0.02\,\delta_{b,f} + 0.91\,\delta_{b,g}, \qquad (40)\\
\epsilon_{f\to b} &= 0.07\,\delta_{b,g} + 0.035\,\delta_{b,e} + 0.90\,\delta_{b,f},
\end{aligned}$$

where the Kronecker $\delta_{b,a} = 1$ iff $a = b$ and $\delta_{b,a} = 0$ otherwise.


[1] S. Haroche and J.M. Raimond, *Exploring the Quantum: atoms, cavities and photons*, Oxford University Press, Oxford (2006).

[2] B. Peaudecerf, C. Sayrin, X. Zhou, T. Rybarczyk, S. Gleyzes, I. Dotsenko, J. M. Raimond, M. Brune, and S. Haroche, *Quantum feedback experiments stabilizing Fock states of light in a cavity*, Phys. Rev. A **87**, 042320 (2013).

[3] V. Métillon, S. Gerlich, M. Brune, J.M. Raimond, P. Rouchon, and I. Dotsenko, *Benchmarking maximum-likelihood state estimation with an entangled two-cavity state*, Phys. Rev. Lett. **123**, 060404 (2019).
